# Supplementary material for: Theory-guided Data Science: A New Paradigm for Scientific Discovery from Data
Source: arXiv:1612.08544 source file (2017-11-13)
Supplement: Supplementary file 1 [file appendix.tex]

%!TEX root = ../main_file.tex

\section{Ansu's original write-up}
Most spatio-temporal datasets are indexed by (two or three dimensional) spatial variables $s = (s_{1}, \ldots, s_{\ell})$ and positive reals $t$. The observations are on a collection of features $Y (s, t) \in \mathbb{R}^{d}$. In many situations, the data may be collected on regular points of a spatial grid, or at regular intervals of time, which renders parts or all of the indexing set to be discrete. Many studies consider only univariate feature of interest, this $d = 1$, although very often co-variables $\mathbf{x} (s, t) \in \mathbb{R}^{p}$ are associated with $Y (s, t)$.

Several challenges abound in these kinds of data. The three dimensional case has has special mathematical challenges arising from the transience of Brownian motion \cite{morters2010brownian}. Data on one or more features at multiple spatial locations and time instances may be missing or unobserved. In physical systems, such lack of data may be owing to the the potential value of the data itself, so a {\it missing at random} assumption may not be appropriate. For example, the truncation of absence of data on the height of a river may be due to a potential flood or drought condition, which may itself be the object of study. Not accounting for truncation, censoring, or missing-not-at-random properties of the data may lead to biased results, and greatly affect precision and accuracy statements. More dangerously, it can potentially lead to policy decisions that may affect future outcomes in unintended ways. Since future measurements may be made without awareness of potential bias and inaccuracy in current data, such inaccuracies may not be identified till considerable harm has been done.

Very often, the mean and the variance of $Y (s, t)$ are under study, as functions of space $s$, time $t$, co-variables $\mathbf{x} (s, t)$, see \cite{currie2006generalized} for a standard approach. However, it is conceivable that other functionals of the distribution of $Y (s, t)$, like quantiles or probabilities, may be of relevance in several practical problems. The most common approach for spatio-temporal modeling as well as smoothing involves assumptions of Gaussian random field for the feature $Y (s, t)$, and much attention is given to specifying parameter structures of such random fields. Since a fully accurate specification is often impossible and because Bayesian statistical methods are commonly in use, hierarchical model specification is also common in spatio-temporal modeling. The papers \cite{katzfuss2011spatio, katzfuss2012bayesian} present examples of this kind of models on massive remote sensing data. They also point out the utility of using dimension reduction methods, and on the use of discretization of partial differential equations and integro-difference equations, for which further references are \cite{cressie2011statistics, wikle2003hierarchical, cangelosi2009models, stroud2010ensemble}. Further details may be found in \cite{cressie2011statistics}. Dimension reduction methods like the above may also be used to incorporate domain knowledge driven regulations and constraints.

In general, hierarchical Bayesian modeling is compatible with domain guided restrictions on the model. These are usually incorporated as part of the {\it prior specification}. Most modern Bayesian models require extensive computation for the extraction of a sample from the posterior distribution, and domain-guided knowledge and constraints may result in loss of speed and efficiency of computational algorithms. Another alternative is to use penalization methods appropriately, ses for example \cite{lee2011p}. Similar approaches have been used for longitudinal and mortality data by \cite{biatat2011hierarchical}, and for flexible regression in river systems by \cite{odonnell2014flexible}.

A large body of literature assume a {\it separable} form, where spatio-temporal dependence is factorizable into two parts, one a function space only and another a function of time \cite{macnab2001autoregressive, kneib2006structured}. However, non-separable models may be better representative of the properties of the data and physical system under study.

\section{Socially-relevant ML}
In past decade, data science has grown significantly to not only push the boundaries of computer science but has flourished in a wide-range of applications. However, amid data science's rapid growth, the field has become adept at solving a narrow set of problems, while largely ignoring others, especially socially relevant ones. \cite{wagstaff2012machine, faghmous2013stdm, Ganguly2014, rudin2014machine, Faghmous2014Big, Faghmous2014IEEE}. While there are many things to celebrate about the growth of data science there is an equal need to create new environments where novel applications of data science can flourish.

\section{Problem-First Statistics}
One such application is that of addressing climate change where the singular combination of unique data, challenging scientific questions, and urgent societal needs make it a great opportunity for pioneering research. This line of work seeks to return to the root of the field of data science: where pressing societal needs fueled the development of modern statistics. For the works of John Graunt studying plague in England \cite{grauntnatural}, Laplace's work , Florence Nightingale (The Royal Statistical Society's first female member) works in epidiomoiogy, Arthur Bowley's work on census \cite{bowley1936new}, and perhaps most famously Ronald Fisher's works on crops \cite{fisher1934statistical} have all contributed to the foundation of what is known today as statistics and experiment design. This suggests that innovation can be facilitated through urgent social questions and not only novel methods.

\section{Data science}

\subsection{broad over-view}
During the same period of data science's growth, numerous scientific domains such as Earth science and neuroscience rapidly became inundated with data. Yet, these domains faced challenges that were unknown to traditional data science. First, the data had three starkly different characteristics: (i) they were noisy, incomplete, and heterogeneous; (ii) they were spatio-temporal; (iii) and although their volume was large the number of samples did not rival the scales provided by the Internet. A second significant difference, was that these fields driven by scientific insight were more interested in knowledge rather than accuracy. Hence, highly flexible yet ``black box'' models were not an option. These two factors made it such that any out-of-the-box application of existing methods would yield limited insight.

\subsection{Internet-scale data science is incremental}
One view on Internet-scale data science is that it is a natural evolution from the industrial-scale society. When we needed to scale our output as a society, assembly-lines were created, 1-to-many classroom educational systems were built. Today, the next scale is millions of people, hence Internet-scale data science is simply a step in the same direction. More importantly, what we are learning in the age of ``Big Data'' first, there are numerous problems that cannot be solved with scale alone.

\subsection{Comments on learning}
One can argue that humans are the most sophisticated data processors in the world. We are constantly collecting data from our sensory system and processing and reacting to them, in real-time, using our cognitive system. Yet, despite being the most advanced data processing entity we have yet to discover, humans have numerous cognitive limitations that result in sub-optimal or even irrational behaviors.

This reality has led to two different, yet complimentary, developments in the broad computational sciences community. On one side, we took the ``imitation is the best form flattery'' route where our fascination with human cognitive abilities led to the development of a wide-range of efforts seeking to reproduce human biological or cognitive capabilities from the Turing test to biologically-inspired hardware. On the other side, scientists sought to ``augment'' human capabilities by using data to make us better (healthier, smarter, \emph{etc.}) While both approaches have tremendous merits, we are starting to see a disproportional focus on the former research agenda of allowing machines to mimic tasks that are trivial to humans, yet have proven extremely difficult for machines.

\subsection{Is there a bubble?}
In recent years there has been a lot of speculation whether we are in an ``Internet bubble'', due to the astronomically high valuations unproven Internet startups were receiving (as well as high-priced acquisitions). However, some have argued that even if there is a bubble any negative effects of its bursting would be isolated to Silicon Valley \cite{Lowrey2014}. While that might be true, Silicon Valley has a disproportionate and long-lasting effects on how data science evolves and the areas we ought to focus on.

\begin{figure}[htbp]
	\centering
	\includegraphics[width=0.50\textwidth]{figures/fire_example.pdf}
	\caption{Analyzing phenomena in space and time provides richer information than any one dimension alone. Left and middle panels show the forest cover before and after a 2008 fire in Big Sur, California, USA. The right panel shows temporal changes in a vegetation proxy variable (EVI) at a location within the fire.}
	\label{fig:fire_example}
\end{figure}

\subsection{Broad trends in data science}
The science of extracting knowledge from data using statistical, machine learning, and data mining techniques (data science) is a broad and rapidly evolving field. However, a large portion of present-day data science has been shaped by three major trends that have guided its direction and focus as a field of knowledge.
In their classic paper, Fayyad, Piatetsky-Shapiro, and Smyth \cite{fayyad1996data} outlined the \emph{Knowledge Discovery in Databases (KDD) process} -- a seven-step procedure that went from data to knowledge. The authors highlighted the fact that data mining is \emph{a step} in the KDD process and not the end itself. That is, the goal of the process was the discovery of novel, useful, and non-trivial knowledge. However, the field of machine learning has been a dominant player in data science's recent evolution. Machine learning has been defined as ``algorithms that improve their performance as more data are observed'' [need citation for this]. This definition has become the driving force of major research academic conferences where the focus has become more on the the development of algorithms or methods (i.e. the data mining step in the KDD process) rather than knowledge discoveries \cite{Langley2011,wagstaff2012machine}. A methods-centric approach enabled rapid growth for the discpline of data science, and we have made significant progress in several computational problems (e.g. computer vision, recommendations, collaborative filtering, \emph{etc.}). The methods innovation cycle was accelerated by the launch of the UCI Machine Learning Repository, which hosted various benchmark datasets that could be used to objectively compare algorithm performance. Furthermore, and in order to compare methods, objective yet abstract, metrics such as root mean squared error (RMSE) became \emph{de facto} evaluation metrics. While these focused developments led to rapid growth, it also narrowed the types of problems data science tackled to mainly classification, regression, and ranking tasks. More recently, we are also witnessing the wide-spread popularity of ``Big'' data science, where the task is to learn from billions or trillions of observations fueled by Internet-scale datasets, mainly from large Internet companies. In fact, today Internet companies are commonly ranked as top data mining institutions ahead of research universities \footnote{See Microsoft Academic Research: \url{http://academic.research.microsoft.com/RankList?entitytype=7&topDomainID=2&subDomainID=7&last=0&start=1&end=100}}. While these large datasets have driven significant innovations, they tend to focus primarily on tasks of interest to Internet companies such as content recommendation, facial recognition, or identifying objects within an image. While all these developments have been significant and timely, they have gotten a disproportionate amount of attention and resources compared to other pressing needs. As a result, the methods-centric approach, the narrow focus on certain data problems such as classification, and the string influence Internet companies have had in determing the data science research agenda have left us unprepared to tackle significant data-driven challenges of momentous societal and scientific interest.

\subsection{Spatio-Temporal Data Analysis as The New Inference Frontier}
Although one of the primary goals of data-driven methods is to infer causality \cite{pearl1988probabilistic}, a significant challenge of the ``Big Data era'' is to separate correlation and causation \cite{wright1921correlation}. Spatio-temporal data allow us to contextualize our data analysis and understand processes in better detail. The basic truism that``there is no history without geography'' \cite{cressie2011statistics} underscores the crucial need for spatio-temporal analysis, which facilitates inference by considering space and time together.

Figure \ref{fig:fire_example} shows before and after satellite snapshots of a region that experienced a severe forest fire. Although it might be useful to view before and after snapshots of an event (right and center panels), the observer gains limited insight about the behavior of the changes that occurred over a significant timespan (in this case 6 months). The high-frequency temporal information in the left panel does show the abrupt vegetation loss in 2008 but does not provide the spatial extent of the fire event. Hence, a spatio-temporal analysis of such events would allow better characterization, identification, and prediction than using any one dimension alone.

This research is further motivated by the fact that numerous real-world phenomena are inexorably linked to space and time and it would be impossible to study them without a spatio-temporal framework. For example, it is well-established that hurricanes only form under a distinct set of spatio-temporal conditions \cite{Gray1979}. Similarly, a host of cognitive functions such as addiction respond to spatio-temporal stimuli \cite{bohbot2013caudate}. Finally, recent brain imaging studies also suggest that the brain encodes information based on the spatio-temporal activation patterns of neurons \cite{muto2013real}.

In addition to their promise to enable the study of phenomena as never before, spatio-temporal data are rapidly becoming ubiquitous. Earth orbiting satellites, GPS-enabled phones, even location-aware apparel are contributing to the massive size and variety of spatio-temporal data, and this trend will continue with affordable drones, satellites (\emph{e.g.} CubeSat), and other wearable technology. Thus, developing methods that can cope with the unique characteristics of spatio-temporal data is a sound investment.

\section{Climate sciences}
Global climate change and its impact on human life has become one of our generation's most defining challenges. While the science behind global warming is settled \cite{Stocker2013}, there are significant knowledge gaps about how extreme events such as droughts, hurricanes, and floods might respond to significant changes to our climate (known broadly as \emph{climate change impacts}). Although complex climate model simulations are the primary tool for understanding climate change, a leading source of uncertainty is their inability to resolve many of the climate impact phenomena of interest at spatio-temporal scales that matter to stakeholders (local communities, policy makers, etc.) \cite{Field2014}. These climate model limitations, both theoretical and computational, are expected to persist for the next decade \cite{stevens2013climate}, during which, climate science will continue to experience exponential data growth \cite{overpeck2011} and is expected to output hundreds of exabytes (1 exabyte = 1,000 petabytes) by 2020 \cite{williams2013earth}.

Climate science is the study of our planet's environment. Our planet is the most splendid example of a complex dynamical system in perpetual motion to balance energy and sustain its habitable environment. Fundamentally, climate science is a field focused on studying large-scale changes in the land, atmosphere, oceans, and cryosphere over long temporal periods (years, decades, centuries). Although, some consider shorter (weather) time-scales such as days or weeks to also be part of the studying climate. Figure 1, shows a more complex view of the climate system. The interacting parts of the system range from micrometer-sized particles and aerosols to large-scale changes in the land surface.  What is missing from Figure 1 is a notion of the temporal scales at which these interactions occur. Some interactions might last hours or days -- such as the influence of sea surfaces temperature on the formation of a hurricane -- while other interactions might occur over several years (e.g. ice sheets melting). Thus it is not only important to know the interacting parts of the system, we must also understand the spatio-temporal scales at which they interact.

Monitoring these constantly evolving planetary patterns is critical for us to understand what drives the above-mentioned interactions and how they might change if the planet continues to warm. The idea is to understand what drives certain planetary processes and then project any changes in theses processes if some of the drivers changed (e.g. because of increased greenhouse gas emissions.)

On the surface, such predictive modeling and casual inference are common exercises in traditional data science. So why is data science's impact on climate science lagging that of other domains? There are three major factors that have slowed progress. First, the data that climate science uses violates many of the assumptions and practices held in traditional data science. For example, the majority of climate data tend to be organized in a spatio-temporal grid. As such, the data tend to be auto-correlated where regions in spatial or temporal proximity tend to be highly related. Hence, any methods that impose independence assumptions amongst data points will have limited practicality with such data. Second, the field of data science has historically focused on certain tasks and evaluation metrics. However, those learning and evaluation tasks are not applicable to some of climate science's biggest needs. Finally, and this is only a matter of time, but climate science, its data, and challenges have not been exposed to the broader data science community until recently. However, the body of work in this domain is steadily increasing and we are also seeing new interdisciplinary centers such as the NSF-funded center on understanding climate change from data at the University of Minnesota and Center for Atmosphere Ocean Science of the Courant Institute of Mathematical Science at New York University. We are also encouraged by the growing communities of computational sustainability and climate informatics.

\section{Parking lot}
\begin{enumerate}
	\item Data science has experienced exponential growth over the past few decades in large part thanks to the Internet. The Internet democratized the creation, distribution, and analysis of data on scales never seen before.
	\item different types of data/information. For example many of these applications are concerned with static data, yet there is tremendous interest in change and rates of change. Rates at which we are transforming the planet are much fasted than our ability to understand it.

	\item Additionally there are some strategies that can be put in place to encourage the trans-disciplinary collaboration needed to foster this much-needed yet overlooked area of data science.

\begin{enumerate}
\item Joint-funding
\item Coalition of laboratories
\item Revisiting publication standards
\item Creating new publication venues
\item Post-doctoral career opportunities
\item Engaging large Internet companies
\item A network of research groups that students can join easily with flexible funding to host students.
\end{enumerate}

\end{enumerate}
